# Supplementary material for: Quantum annealing and non-equilibrium dynamics of Floquet Chern insulators
Source: arXiv:1508.01883 source file (2016-12-27)
Supplement: Supplementary file 1 [file floquet_qa_supp_04.pdf]

# Supplementary Material for
# Quantum annealing and non-equilibrium dynamics of Floquet Chern insulators

Lorenzo Privitera[1], Giuseppe E. Santoro[1,2,3]
[1] *SISSA, Via Bonomea 265, I-34136 Trieste, Italy*
[2] *CNR-IOM Democritos National Simulation Center, Via Bonomea 265, I-34136 Trieste, Italy*
[3] *International Centre for Theoretical Physics (ICTP), P.O.Box 586, I-34014 Trieste, Italy*

We present here a few useful technical aspects of our study. We start by explaining in full detail the calculations that we implemented to solve the Schrödinger dynamics. Next, we discuss the periodic oscillations of the current. We continue by summarizing the main points of Ref. [1] on the local Chern marker $\mathcal{C}(\mathbf{r})$, for the reader's convenience; we then discuss the results for the quantum annealing (QA) dynamics of $\mathcal{C}(\mathbf{r},t)$ both for the Haldane model, and for the irradiated graphene model. Finally, we present animations showing how the case of a perturbation of frequency $\omega$ smaller than the unperturbed bandwidth $W$ is intriguingly "non-adiabatic": the standard Kibble-Zurek (KZ) scenario is inappropriate, and important excitations inside the bulk quasi-energy bands occur.

**QA dynamics of Slater determinants.**

We outline here the main steps involved in doing QA dynamics of the Hamiltonian in Eq. 1 of the main paper. The crucial ingredient is that an initial Slater determinant remains a Slater determinant under an arbitrary unitary time-evolution, as long as the driving Hamiltonian is quadratic in the fermionic operators. In our implementation, we have considered a zig-zag strip with periodic boundary conditions (PBC) in the $y$-direction, and label sites with two integers, $\mathbf{r}_{i,j}$ with $i = 1\cdots N_x$ and $j = 1\cdots N_y$, along zig-zag lines at 30° from the $x$-direction (see inset of Fig. 2-$\mathbf{b}'$ of the main text). In terms of the nearest-neighbor (nn) vector $\mathbf{d}_2 = d(\frac{1}{2}\hat{\mathbf{x}} + \frac{\sqrt{3}}{2}\hat{\mathbf{y}})$ and the lattice vector $\mathbf{a}_1 = a(\frac{\sqrt{3}}{2}\hat{\mathbf{x}} + \frac{1}{2}\hat{\mathbf{y}})$ we then write: $\mathbf{r}_{1,1} = \mathbf{0}$, $\mathbf{r}_{2,1} = \mathbf{d}_2$, and $\mathbf{r}_{i\geq 2,j} = \mathbf{r}_{i-2,1} + \mathbf{a}_1 + a(j-1)\hat{\mathbf{y}}$. We assume the strip width $N_x$ to be even, and the origin to belong to the $\mathcal{A}$-sublattice. Translational invariance along $y$ allows using $k$ as a quantum number, introducing Bloch transformations

$$\hat{c}^\dagger_{i,k} = \frac{1}{\sqrt{N_y}} \sum_{j=1}^{N_y} \mathrm{e}^{ikaj} \hat{c}^\dagger_{i,j} \;,$$

with $ka = \frac{2\pi n}{N_y}$ $(n = 0, \cdots, N_y - 1)$ in terms of which the Hamiltonian in Eq. 1 of the main text can be expressed as:

$$\hat{H}(t) = \sum_k^{\mathrm{BZ}_y} \sum_{i,i'=1}^{N_x} \mathbb{H}_{ii'}(k,t)\; \hat{c}^\dagger_{i,k}\hat{c}_{i',k} \;. \tag{1}$$

Here $\mathbb{H}(k,t)$ is an $N_x \times N_x$ Hermitean matrix with elements on the diagonal (the on-site terms) and at nn (for the Haldane model there are also second-neighbor terms). The initial Slater determinant $|\Psi(0)\rangle$ is constructed by diagonalizing $\mathbb{H}(k,0)$ for each $k$, obtaining the eigenvectors $u_{i,\alpha}(k)$ and forming the corresponding eigenmode combinations $\hat{a}^\dagger_{\alpha,k} = \sum_i u_{i,\alpha}(k)\,\hat{c}^\dagger_{i,k}$, which are then occupied according to Pauli principle. Any relevant translationally invariant operator can be decomposed in terms of the Bloch combinations $\hat{c}^\dagger_{i,k}$. For instance, the $y$-component of the current flowing along the bond $(\mathbf{r}_{i,j}, \mathbf{r}_{i',j})$, averaged over $j$, — for the Haldane case there are also second-neighbor currents along bond $(\mathbf{r}_{i,j}, \mathbf{r}_{i,j+1})$ — can be expressed as:

$$\hat{J}_{ii'}(t) = \sum_k^{\mathrm{BZ}_y} \mathbb{J}_{ii'}(k,t)\; \hat{c}^\dagger_{i,k}\hat{c}_{i',k} \;, \tag{2}$$

with $\mathbb{J} = \frac{1}{\hbar}\frac{\partial \mathbb{H}}{\partial \kappa_y}\Big|_{\kappa_y=0}$, where $\kappa_y = \frac{2\pi}{aN_y}\frac{\Phi_L}{\phi_0}$ is related to the Laughlin flux $\Phi_L$, in units of the flux quantum $\phi_0$, piercing the PBC-cylinder along the $x$-axis. If $|\Psi(t)\rangle$ denotes the time-evolved Slater determinant state of the system, then all physically relevant observables can be extracted from the knowledge of the single-particle Green's function:

$$\mathbb{G}_{i'i}(k,t) \equiv \langle \Psi(t)|\hat{c}^\dagger_{i,k}\hat{c}_{i',k}|\Psi(t)\rangle \;. \tag{3}$$

Equivalently, in the Heisenberg representation, $\mathbb{G}_{i'i}(k,t) = \langle \Psi(0)|\hat{c}^\dagger_{i,k}(t)\hat{c}_{i',k}(t)|\Psi(0)\rangle$. The Schrödinger unitary dynamics implies a simple linear equation of motion for the Heisenberg's operators $\hat{c}^\dagger_{i,k}(t)$ and $\hat{c}_{i',k}(t)$, which can be solved as follows. The initial eigenstate wavefunctions at given $k$ are conveniently organized into an $N_x \times N_x$ unitary matrix $\mathbb{S}^0(k) = [u_{i,\alpha}]$, with $k$-eigenvectors by columns. One can show that the Heisenberg's equations for $\hat{c}_{i,k}(t)$ are solved by $\hat{c}_{i,k}(t) = \sum_\alpha \mathbb{S}_{i,\alpha}(k,t)\,\hat{a}_{\alpha,k}$, where the matrix $\mathbb{S}(k,t)$ obeys the Schrödinger equation:

$$i\hbar\frac{d}{dt}\mathbb{S}(k,t) = \mathbb{H}(k,t)\cdot\mathbb{S}(k,t) \;. \tag{4}$$

This matrix differential equation is solved, for each $k$, with initial value $\mathbb{S}(k,0) = \mathbb{S}^0(k)$, through a standard $4^{th}$-order Runge-Kutta numerical integration. The integration is carried-on up to time $t = \tau_{\rm QA} = n_{\rm QA}\tau$ where the adiabatic switching-on of the periodic perturbation is completed; we take $\tau_{\rm QA}$ to be an integer multiple $n_{\rm QA}$ of the period of the driving $\tau = 2\pi/\omega$. Following that, we carry-on an evolution governed by the final periodic Hamiltonian with fixed $\lambda_{\rm f}$ for a time $\tau_{\rm f} = n_{\rm f}\tau$; the unitary evolution operator allows us to write, at any later time, $\mathbb{S}(k,t) = \mathbb{U}_k(t, n_{\rm QA}\tau)\,\mathbb{S}(k, n_{\rm QA}\tau)$. This periodic evolution is greatly simplified by using the Floquet theorem, which guarantees that the evolution operator $\mathbb{U}_k(t, n_{\rm QA}\tau)$ can be written as $\mathbb{U}_k(t, n_{\rm QA}\tau) = \mathbb{U}_k(\delta t, 0)[\mathbb{U}_k(\tau, 0)]^n$, where $t = (n+n_{\rm QA})\tau + \delta t$ with $0 \le \delta t < \tau$. The evolution operator over a period $\mathbb{U}_k(\tau, 0)$, the so-called Floquet operator, plays then a crucial role: its eigenvectors are the Floquet modes $|\phi_{k,\alpha}(0)\rangle$, with phase-eigenvalues $\mathrm{e}^{-iE_{k,\alpha}\tau/\hbar}$ expressed in terms of quasi-energies $E_{k,\alpha}$. The resulting periodic dynamics can be then followed up to large times by simply solving the one-period Floquet problem. Once $\mathbb{S}(k,t)$ is constructed, the physical Green's function is obtained from:

$$\mathbb{G}_{i'i}(k,t) = \sum_{\alpha}^{\rm occ} \mathbb{S}_{i'\alpha}(k,t)\; \mathbb{S}^{\dagger}_{\alpha i}(k,t)\ . \qquad (5)$$

The Green's function $\mathbb{G}_{i'i}(k,t)$ directly provides a real-space representation for the projector $\mathcal{P}(t)$ on occupied states used in the construction of the Chern marker $\mathcal{C}(\mathbf{r})$ (see below):

$$\langle \mathbf{r}_{i',j'}|\mathcal{P}(t)|\mathbf{r}_{i,j}\rangle = \frac{1}{N_y}\sum_{k}^{{\rm BZ}_y} \mathrm{e}^{-ika(j-j')}\;\mathbb{G}_{i'i}(k,t)\ . \qquad (6)$$

### Expectation values of the current operator

In periodically driven systems with a continuous Floquet spectrum it is often found that, starting from a generic state $|\Psi(0)\rangle$, the expectation values of the observables oscillate in a periodic fashion, after a suitable transient time[2, 3]. The asymptotic limit of observables calculated at stroboscopic times $t^* + n\tau$, where $\tau$ is the period and $t^* \in [0,\tau]$, are captured, for very large $n$, by their Floquet *diagonal* averages [2, 4]. For the $y$-current we have

$$\langle \hat{J}\rangle_{\rm diag}(t^*) = \sum_{\alpha}\int_0^{\frac{2\pi}{a}} \frac{\mathrm{d}k}{2\pi}\; n_{k,\alpha}\; \mathbb{J}_{\alpha\alpha}(k,t^*) \qquad (7)$$

where $n_{k,\alpha}$ is the occupation of the $\alpha$-th Floquet mode $|\phi_{k,\alpha}(t)\rangle$, and we have introduced a shorthand $\mathbb{J}_{\alpha\alpha}$ for the diagonal matrix element of the current operator in the Floquet basis:

$$\mathbb{J}_{\alpha\alpha}(k,t^*) = \langle \phi_{k,\alpha}(t^*)|\hat{J}(k,t^*)|\phi_{k,\alpha}(t^*)\rangle\ .$$

The occupations are calculated from

$$n_{k,\alpha} = \langle \Psi(n\tau)|\hat{f}^{\dagger}_{k,\alpha}\hat{f}_{k,\alpha}|\Psi(n\tau)\rangle\ , \qquad (8)$$

where $\hat{f}^{\dagger}_{k,\alpha} = \sum_i \phi_{k,\alpha}(i)\hat{c}^{\dagger}_{i,k}$ is the operator that creates an electron in the Floquet mode $|\phi_{k,\alpha}\rangle$, and $|\Psi(n\tau)\rangle$ the time-evolved Slater determinant at stroboscopic time $n\tau$, with $n > n_{\rm QA}$. The matrix element of the current, in turn, can be written as [5]

$$\mathbb{J}_{\alpha\alpha}(k,t) = \frac{1}{\hbar}\frac{\partial E_{k,\alpha}}{\partial k} + \frac{\partial}{\partial t}\langle \phi_{k,\alpha}(t)|\partial_k \phi_{k,\alpha}(t)\rangle\ , \qquad (9)$$

where $E_{k,\alpha}$ is the *quasi-energy* of the Floquet mode $|\phi_{k,\alpha}(t)\rangle$. Since the Floquet modes are $\tau$-periodic, the average of the matrix element over one period reads

$$\Big[\mathbb{J}_{\alpha\alpha}(k,t)\Big]_{\rm av} = \frac{1}{\hbar}\frac{\partial E_{k,\alpha}}{\partial k}\ . \qquad (10)$$

Hence, upon averaging over the periodic oscillations, the total asymptotic current turns out to be:

$$\Big[\hat{J}\Big]_{\rm av} = \sum_{\alpha}\int_0^{\frac{2\pi}{a}} \frac{\mathrm{d}k}{2\pi}\; n_{k,\alpha}\frac{1}{\hbar}\frac{\partial E_{k,\alpha}}{\partial k}\ . \qquad (11)$$

This expression resembles the corresponding one for an equilibrium time-independent $\hat{H}$, with quasi-energies playing the role of the energy eigenvalues. However, as illustrated in the main text in Fig. 2-**a′**, there are in general large periodic oscillations of the current — often referred to as "micro-motion" — typically much bigger than their average value.

### The local Chern marker of Bianco & Resta.

The Hall conductance of a two-dimensional insulator (in the perfect infinite crystal limit) can be written in terms of a Berry curvature and Chern number $\mathcal{C}$ [6, 7] as $\sigma_{yx} = \frac{e^2}{h}\mathcal{C}$ where:

$$\begin{aligned}\mathcal{C} =& \frac{i}{2\pi}\sum_{p}^{\rm occ}\sum_{q}^{\rm unocc}\int_{\rm BZ} d\mathbf{k}\Big(\langle \partial_{k_x}u_{p\mathbf{k}}|u_{q\mathbf{k}}\rangle\langle u_{q\mathbf{k}}|\partial_{k_y}u_{p\mathbf{k}}\rangle - \text{c.c.}\Big)\\ =& 2\pi i\sum_{p}^{\rm occ}\sum_{q}^{\rm unocc}\int_{\rm BZ}\frac{d\mathbf{k}}{(2\pi)^2}\Big(\left(\hat{x}_{\mathcal{P}}(\mathbf{k})\right)_{pq}\left(\hat{y}_{\mathcal{Q}}(\mathbf{k})\right)_{qp} - \text{c.c.}\Big)\\ =& 2\pi i\ \mathrm{Tr}\Big(\hat{x}_{\mathcal{P}}\hat{y}_{\mathcal{Q}} - \hat{y}_{\mathcal{P}}\hat{x}_{\mathcal{Q}}\Big)\ .\end{aligned}$$

Here $|u_{p/q\,\mathbf{k}}\rangle$ denote the periodic part of a set of occupied/empty Bloch states. The second form is obtained by using $\langle \partial_{k_x}u_{p\mathbf{k}}|u_{q\mathbf{k}}\rangle = -\langle u_{p\mathbf{k}}|\partial_{k_x}u_{q\mathbf{k}}\rangle$ and re-expressing the result in terms of momentum-space matrix element of the position operators $\hat{x}_{\mathcal{P}} = \mathcal{P}\hat{x}\mathcal{Q}$ and $\hat{y}_{\mathcal{Q}} = \mathcal{Q}\hat{y}\mathcal{P}$ sandwiched between the projectors $\mathcal{P}$ and $\mathcal{Q}$ on occupied and empty bands: $\left(\hat{x}_{\mathcal{P}}(\mathbf{k})\right)_{pq} = \langle u_{p\mathbf{k}}|i\partial_{k_x}u_{q\mathbf{k}}\rangle$ and

$(\hat{y}_{\mathcal{Q}}(\mathbf{k}))_{qp} = \langle u_{q\mathbf{k}} | i\partial_{k_y} u_{p\mathbf{k}} \rangle$. The final form makes it explicit that the sums over $p$ and $q$ and the momentum space integral yield simply a *trace* expression in terms of projected position operators. Now the crucial step [1] consists in realizing that the trace can be calculated in any representation. Hence, switching to real space we can extract a *local Chern marker* (CM) $\mathcal{C}(\mathbf{r})$ as:

$$\mathcal{C}(\mathbf{r}) = 2\pi i \langle \mathbf{r} | \Big( \hat{x}_{\mathcal{P}} \hat{y}_{\mathcal{Q}} - \hat{y}_{\mathcal{P}} \hat{x}_{\mathcal{Q}} \Big) | \mathbf{r} \rangle \ , \tag{12}$$

in terms of which $\mathcal{C} = \lim_{V\to\infty} \frac{1}{V} \int_V d\mathbf{r} \ \mathcal{C}(\mathbf{r})$. This local expression can be used also for an open boundary (OB) geometry, and even when translational invariance is broken by disorder. Interestingly, when one considers open boundary conditions (OBC), where $\hat{x}$ and $\hat{y}$ are well defined operators even without projectors [8], we can rewrite $\mathcal{C}(\mathbf{r})$ in a more appealing form in terms of standard commutators[1]. Indeed $\hat{x}_{\mathcal{P}} \hat{y}_{\mathcal{Q}} - \hat{y}_{\mathcal{P}} \hat{x}_{\mathcal{Q}} = \mathcal{P}(\hat{x}\mathcal{Q}\hat{y} - \hat{y}\mathcal{Q}\hat{x})\mathcal{P} = -[\hat{x}_{\mathcal{P}}, \hat{y}_{\mathcal{P}}]$, where we used $\mathcal{Q} = 1 - \mathcal{P}$, $[\hat{x}, \hat{y}] = 0$, and standard properties of projectors. Hence, a physically equivalent way of writing the local Chern marker is:

$$\mathcal{C}(\mathbf{r}) = -2\pi i \langle \mathbf{r} | \Big[ \hat{x}_{\mathcal{P}}, \hat{y}_{\mathcal{P}} \Big] | \mathbf{r} \rangle \ , \tag{13}$$

which involves the *commutator* of $\mathcal{P}$-projected position operators. Clearly, in this last form, $\int_V d\mathbf{r} \ \mathcal{C}(\mathbf{r}) = 0$, but the local "bulk" physics is well reproduced, due to "Kohn's nearsightedness" of electrons in insulators [9]. This form of $\mathcal{C}(\mathbf{r})$ is somewhat evocative of the Bott's index expression [10] used in [11], but a precise matching of the two approaches is lacking.

*Dynamics of the Chern marker*

In order to further clarify the nature of the dynamical topological transition we compare the results already presented in the main text for the Floquet case with those obtained in the simpler case of the Haldane model. The behavior of the local CM is captured by its macroscopic average in the bulk [1], i.e.

$$C_{\text{bulk}}(t) = \frac{1}{N_{\text{bulk}}} \sum_{\mathbf{r}\in\text{bulk}} \mathcal{C}(\mathbf{r}, t) \ . \tag{14}$$

Fig. 1-**a** illustrates the time evolution of $C_{\text{bulk}}(t)$, in the Haldane case, along the evolution arrow of Fig. 1-**a** of the main text, for $L = N_x = N_y = 48$, by considering the bulk portion to be a central square of size $12 \times 12$. Starting from zero, $C_{\text{bulk}}(t)$ begins to grow near the equilibrium topological transition, until it reaches a value $\simeq 0.98$. Afterwards, it fluctuates very weakly around this final value. We find that the time-average of $C_{\text{bulk}}(t)$

$$C^{\text{av}}_{\text{bulk}}(L, \tau_{\text{QA}}) = \frac{1}{\tau_{\text{f}}} \int_{\tau_{\text{QA}}}^{\tau_{\text{QA}}+\tau_{\text{f}}} \text{d}t \ C_{\text{bulk}}(t)$$

reaches, for long annealing times $\tau_{\text{QA}}$, the value corresponding to the ground state of the final Hamiltonian, $C^{\text{eq}}_{\text{bulk}}$, which, in turn, approaches 1 as the size $L$ increases, as shown in Fig. 1-**c**. Moreover, the amplitude of the time fluctuations

$$C^{\text{rms}}_{\text{bulk}}(L, \tau_{\text{QA}}) = \sqrt{\frac{1}{\tau_{\text{f}}} \int_{\tau_{\text{QA}}}^{\tau_{\text{QA}}+\tau_{\text{f}}} \text{d}t \ \left( C_{\text{bulk}}(t) - C^{\text{av}}_{\text{bulk}} \right)^2}$$

goes to 0 as $\tau_{\text{QA}} \to \infty$, see Fig. 1-**b**. These facts shed a light on the nature of the adiabatic transition. As explained in the main text, excitations of the bulk states are of the standard KZ-type and can be controlled by making the annealing time $\tau_{\text{QA}}$ larger and larger, while edge states are occupied in a characteristic non-equilibrium way no matter how large $\tau_{\text{QA}}$ is. However, due to the localized nature of an insulating state [7, 9], the bulk "does not know" about the excited edge states. Thus $C^{\text{av}}_{\text{bulk}} \sim 1$ signals that the bulk correlations are of the insulating type, and that the time-evolved state has managed to follow the instantaneous ground state also in its topological aspects, contrary to what might be expected on the basis of the conservation the total Chern number [11]. When the annealing time is too short, $C^{\text{av}}_{\text{bulk}}$ fluctuates strongly around some value between 0 and 1, indicating that the bulk should be considered to be in a non-equilibrium "metallic" phase. In the Floquet case, whose main features have already been illustrated in the main text, we observe that smooth oscillations appear on top of the behavior illustrated for the Haldane case. For instance, Fig. 1-**a**$'$ shows the result (already presented in Fig. 3 of the main text) for the case of a periodically driven insulator with a finite constant $\Delta_{AB} = 0.1|t_1|$ and size $L = N_x = N_y = 48$. Fig. 1-**b**$'$ shows that by increasing the annealing time $\tau_{\text{QA}}$, the time-average $C^{\text{av}}_{\text{bulk}}$ tends to $C^{\text{av}}_{\text{bulk}} \simeq 0.96$, while the time-fluctuation $C^{\text{rms}}_{\text{bulk}}$ settles down to a small but non-vanishing value $C^{\text{rms}}_{\text{bulk}} \sim 0.04$. However, as shown in Fig. 1-**c**$'$, not only $\lim_{L\to\infty} \lim_{\tau_{\text{QA}}\to\infty} C^{\text{av}}_{\text{bulk}}(L, \tau_{\text{QA}}) = 1$, but also $\lim_{L\to\infty} \lim_{\tau_{\text{QA}}\to\infty} C^{\text{rms}}_{\text{bulk}}(L, \tau_{\text{QA}}) = 0$.

**Intra-band excitations: $\hbar\omega < W$.**

It is interesting to consider what happens when the frequency $\omega$ is below the bandwidth, $\hbar\omega < W$. We find that, due to intra-band resonances, the situation cannot be described in terms of a "Floquet ground state" Slater determinant with small KZ-like excitations on top. To better show the qualitative difference between the two situations, we provide three animations showing the instantaneous Floquet quasi-energy bands and the corresponding occupations (denoted by solid circles whose radius is proportional to the occupation) for three situations: 1) (Anim_omega7_a.avi) a frequency $\hbar\omega = 7|t_1| > W$ with $\Delta_{AB} = 0.1|t_1|$ and an evolution which drives

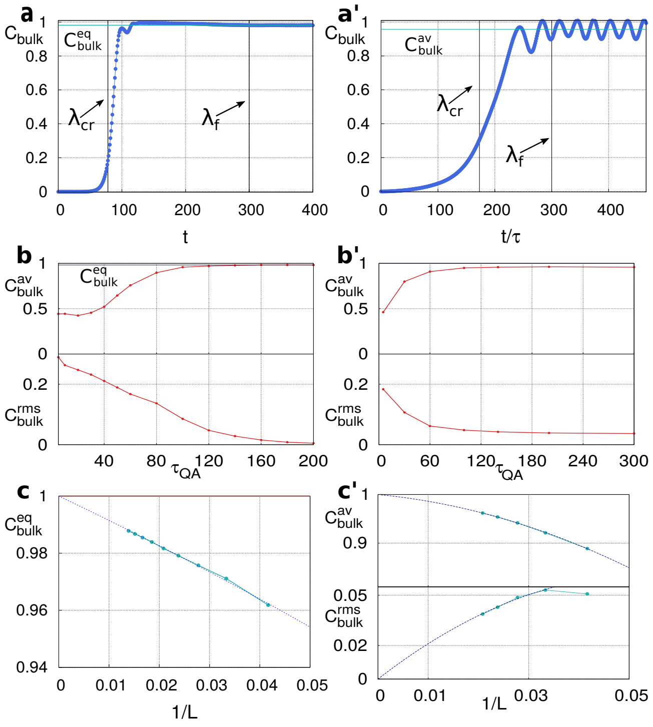


FIG. 1: **Dynamics of the Chern marker.** Bulk Chern marker $C_{\rm bulk}$ for a strip of size $L = N_x = N_y = 48$, calculated on the central square of size $12\times12$ sites, as a function of time, for the Haldane model (**a**, **b** and **c**) and for the graphene-Floquet model (**a′**, **b′** and **c′**). (**a**): Annealing of a Haldane model from $\Delta_{AB}/t_2 = 4\sqrt{3}$ to $\Delta_{AB}/t_2 = 0$, with $\tau_{\rm QA} = 300\tau$, followed by an evolution with $\Delta_{\rm AB} = 0$ for $\tau_{\rm f} = 220\hbar/|t_1|$. The horizontal line at $\approx 0.98$, is the bulk Chern marker of the ground state $C^{\rm eq}_{\rm bulk}$ of the Haldane model with $\Delta_{\rm AB} = 0$. (**b**): the long time average $C^{\rm av}_{\rm bulk}$ of the CM and the long time rms $C^{\rm rms}_{\rm bulk}$ as a function of $\tau_{\rm QA}$ in the Haldane case with the same parameters of (**a**). (**c**): the equilibrium $C^{\rm eq}_{\rm bulk}$ for the Haldane model with $\Delta_{\rm AB} = 0$ versus the size $L$ of the system. (**a′**): Annealing of the driven graphene model with $\lambda(t) = (t/\tau_{\rm QA})\lambda_{\rm f}$ and $\lambda_{\rm f} = 1$, followed by a periodic evolution with fixed $\lambda_{\rm f}$ for $\tau_{\rm f} = 220\tau$; here $\tau_{\rm QA} = 300\tau$, $\hbar\omega = 7|t_1| > W$ and $\Delta_{AB} = 0.1|t_1|$. The horizontal line at $\approx 0.96$ is the long time average $C^{\rm av}_{\rm bulk}$. (**b′**): $C^{\rm av}_{\rm bulk}$ and $C^{\rm rms}_{\rm bulk}$ as a function of $\tau_{\rm QA}$ with the same parameters of (**a′**). (**c′**): $C^{\rm av}_{\rm bulk}$ and the $C^{\rm rms}_{\rm bulk}$ for $\tau_{\rm QA} = 200\tau$ versus $L$. In **a** and **a′**, the first vertical line on the left indicates the closing of the gap in the instantaneous (energy or quasi-energy) spectrum, the second one the end of the annealing. The $C^{\rm av}_{\rm bulk}$ points in **c** and **c′** are fitted by a parabola passing through $(0,1)$, while $C^{\rm rms}_{\rm bulk}$ data are fitted by a parabola passing through $(0,0)$.

$\lambda(t)$ up to the value $\lambda_{\rm f} = 1$ in a time $\tau_{\rm QA} = 100\tau$; 2) (Anim_omega7_b.avi) same as the previous one, but with very small $\Delta_{AB} = 10^{-3}|t_1|$, to effectively represent the case of graphene; 3) (Anim_omega4.avi) a frequency which causes intra-band resonances $\hbar\omega = 4|t_1| < W$, with $\Delta_{AB} = 0.1|t_1|$ and an evolution which drives $\lambda(t)$ up to the value $\lambda_{\rm f} = 1$ in a time $\tau_{\rm QA} = 300\tau$.


[1] R. Bianco and R. Resta, Phys. Rev. B **84**, 241106 (2011).
[2] A. Russomanno, A. Silva, and G. E. Santoro, Phys. Rev. Lett **109**, 257201 (2012), 1204.5084.
[3] A. Russomanno, A. Silva, and G. E. Santoro, J. Stat. Mech. p. P09012 (2013), 1306.2805.
[4] M. Bukov, L. DAlessio, and A. Polkovnikov (2014), arXiv cond-mat.quant-gas/1407.4803v2.
[5] H. Dehghani, T. Oka, and A. Mitra, Phys. Rev. B **91**, 155422 (2015).
[6] Q. Niu, D. J. Thouless, and Y.-S. Wu, Phys. Rev. B **31**, 3372 (1985).
[7] R. Resta, Eur. Phys. J. B **79**, 121 (2011).
[8] R. Resta, Phys. Rev. Lett. **80**, 1800 (1998).
[9] W. Kohn, Phys. Rev. Lett. **76**, 3168 (1996).
[10] T. A. Loring and M. B. Hastings, EPL **92**, 67004 (2010).
[11] L. D'Alessio and M. Rigol, Nat. Commun. **6**, 8336 (2015).
